# Supplementary material for: Exploring the Robustness of Task-oriented Dialogue Systems for Colloquial German Varieties
Source: arXiv:2402.02078 source file (2024-02-03)
Supplement: Supplementary file 1 [file additional_text.tex]

\section{Contrastive evaluation}

\begin{table*}[htp!]
\centering
\resizebox{0.9\textwidth}{!}{ %
\begin{tabular}{lcccc cccc}
\toprule
 & \multicolumn{4}{c}{ \textbf{English VS Perturbed English, UAAVE} } & \multicolumn{4}{c}{ \textbf{German VS Perturbed German} } \\
 &   \xsid &   \atis &  \massive &   \mtop  &   \xsid &   \atis &  \massive &   \mtop  \\ \cmidrule(lr){2-5} \cmidrule(lr){6-9}
\mbert             &  70.55 &  76.04 &    84.14 &  79.72 &  78.01 &  87.57 & 65.97 &  76.77 \\ 
\xlmr              &  67.02 &  79.95 &    70.13 &  82.18 &  83.99 &  90.71 & 75.62 &  85.04 \\
\rembert           &  44.90 &  31.63 &    40.98 &  53.72 &  56.89 &  56.82 & 62.32 &  59.62  \\
\mdeberta          &  46.46 &  50.43 &    59.41 &  49.56 &  71.76 &  64.04 & 63.71 &  74.13 \\ \cdashline{1-9}
\mdistilbert      &  91.40 &  93.99 &    92.05 &  88.67 &  81.56 &  88.31 & 65.75 &  76.26 \\
\mminilm           &  74.33 &  72.87 &    63.93 &  65.59 &  43.96 &  61.57 & 58.25 &  57.58 \\

\bottomrule
\end{tabular}%
    } 
\caption{The average percentage accuracy of language models (LMs) on English (left) and German (right) test sets.  }
\label{tab:pppl_eval}
\end{table*}

Studies on acceptability contrast \cite{song-etal-2022-sling,warstadt-etal-2020-blimp} indicate that a robust LM should yield similar perplexity scores for both the intact sentence and its perturbed version, if the perturbation targets an isolated language phenomena.
In most cases, a robust LM should not prefer one version of the sentence over the other.
Here, we perform a contrastive evaluation by measuring the disparity between perplexity scores on intact sentences and those altered with dialect perturbations.

\noindent \textbf{Preference towards intact sentence.}  We assess the performance of LMs on AAVE and German dialect sentence pairs altered with  individual perturbations using the pseudo-perplexity score \cite{salazar-etal-2020-masked}. 
To estimate accuracy, we calculate the proportion of sentence pairs where the model assigns a higher pseudo-perplexity score to the intact sentence. 
When the accuracy is closer to random guessing (50\%), it indicates that the LM does not show a clear preference between intact and perturbed sentences. 
Higher values indicate LM's preference for intact sentences.

\autoref{tab:pppl_eval} displays the averaged accuracy across all individual dialect perturbation for English and German, respectively.
Overall, LMs exhibit similar behavior, with \rembert and \mdeberta showing slightly better robustness to AAVE perturbations, and \rembert being more robust to German dialect perturbations.  
\mbert and \xlmr strongly favor intact sentences in both languages. 
Distilled models, \mdistilbert  and \mminilm  also show a preference for intact sentences, albeit with lower rates in German. 
The preference for intact sentences is more pronounced in German, peaking at over 90\% with \xlmr.
A key observation is that when the accuracy score in contrastive evaluation is close to a random guess (\atis, \mdeberta) in English, (\atis, \rembert), (\massive, \mminilm) in German, one could expect the performance drop to be less in the fine-tuning setups (\autoref{tab:aave_results}, \autoref{tab:dede_results} in \autoref{sec:tables}). Therefore, LMs generally exhibit a preference towards intact sentences, especially in German, indicating a potential bias towards standard language.
